# Supplementary material for: Unveiling the Mystery of Visual Attributes of Concrete and Abstract Concepts: Variability, Nearest Neighbors, and Challenging Categories
Source: arXiv:2410.11657 source file (2024-10-15)
Supplement: Supplementary file 1 [file Supplementary.pdf]

## Supplementary

**Annotation Study 1 – Difference in Images of Concepts**

As outlined in Section 6.1, we enrolled 13 participants to assess the five identified factors contributing to visual variety in images, utilizing images representing abstract and concrete concepts. For this purpose, we chose two images for each concept from a subset of 18 concepts, specifically including cases that might present challenges. The experiment was carried out using Google Forms. We now showcase examples of how the form looked for participants:

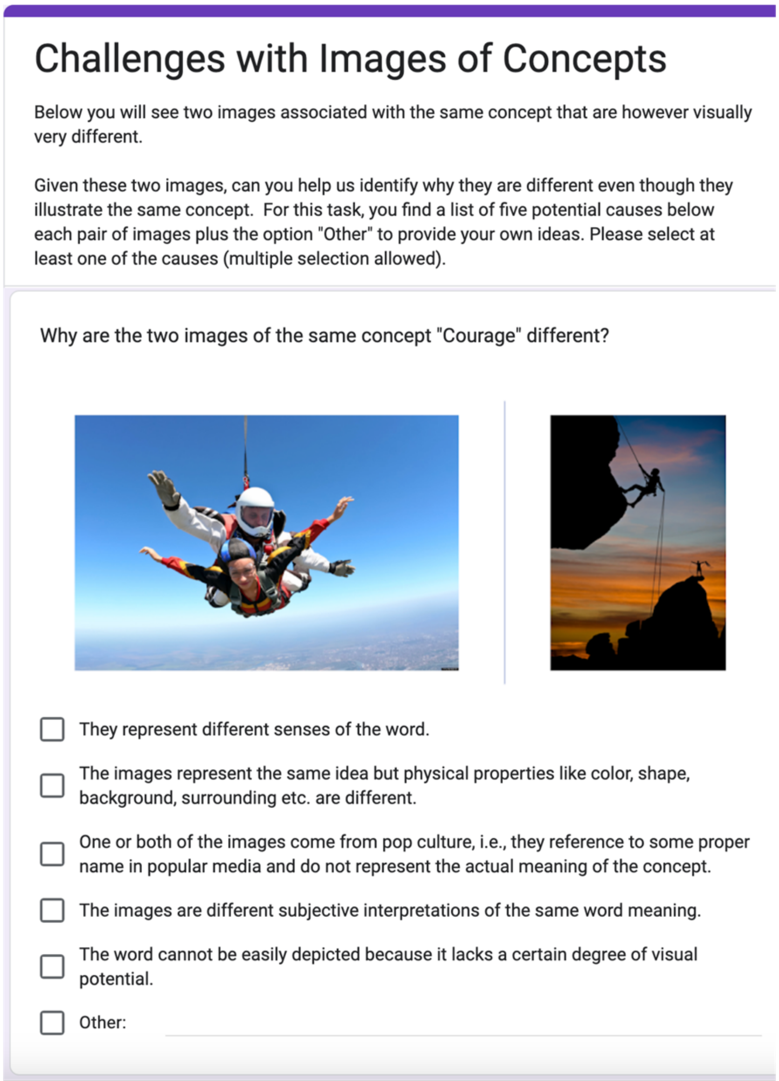

# Challenges with Images of Concepts

Below you will see two images associated with the same concept that are however visually very different.

Given these two images, can you help us identify why they are different even though they illustrate the same concept. For this task, you find a list of five potential causes below each pair of images plus the option "Other" to provide your own ideas. Please select at least one of the causes (multiple selection allowed).

Why are the two images of the same concept "Courage" different?

- [ ] They represent different senses of the word.
- [ ] The images represent the same idea but physical properties like color, shape, background, surrounding etc. are different.
- [ ] One or both of the images come from pop culture, i.e., they reference to some proper name in popular media and do not represent the actual meaning of the concept.
- [ ] The images are different subjective interpretations of the same word meaning.
- [ ] The word cannot be easily depicted because it lacks a certain degree of visual potential.
- [ ] Other:

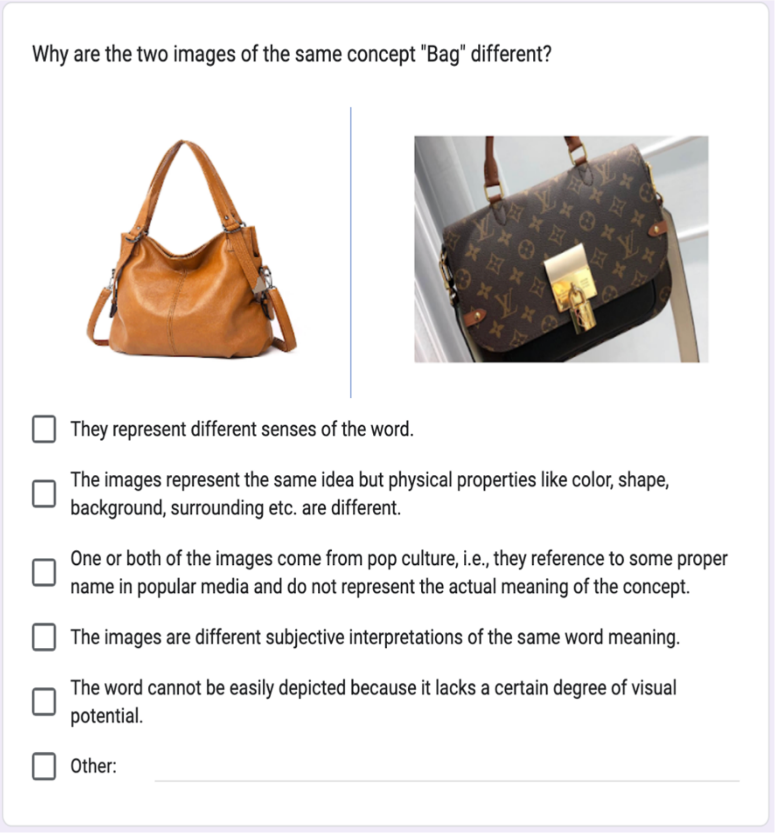
Why are the two images of the same concept "Bag" different?

- [ ] They represent different senses of the word.
- [ ] The images represent the same idea but physical properties like color, shape, background, surrounding etc. are different.
- [ ] One or both of the images come from pop culture, i.e., they reference to some proper name in popular media and do not represent the actual meaning of the concept.
- [ ] The images are different subjective interpretations of the same word meaning.
- [ ] The word cannot be easily depicted because it lacks a certain degree of visual potential.
- [ ] Other:

**Annotation Study 2 – Describing Images**

We further inspect the variability and complexity of diverse but very plausible visual representations of concepts across the 18 images from Study 1 above by conducting a study on Amazon Mechanical Turk study. Participants were tasked with summarizing "what is depicted in each image" using just one word. The participants had to give a minimum of 3 and a maximum of 5 answers.

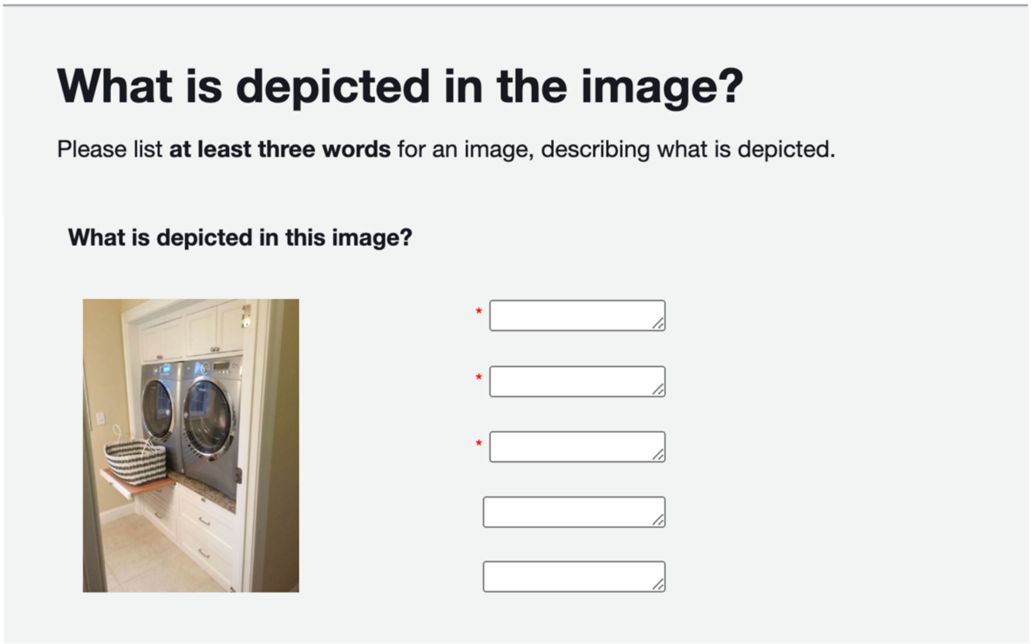
## What is depicted in the image?

Please list **at least three words** for an image, describing what is depicted.

**What is depicted in this image?**

*

*

*
